# Supplementary material for: Algorithm Selection on a Meta Level
Source: arXiv:2107.09414 source file (2021-07-20)
Supplement: Supplementary file 1 [file scenarios.tex]

\documentclass{standalone}
\usepackage{booktabs}
\usepackage{colortbl}
\usepackage{graphicx}

\begin{document}

\definecolor{winner}{RGB}{240,240,240}

\begin{tabular}{llllllllllllll}
                          & \multicolumn{1}{c}{\rotatebox{90}{ASP-POTASSCO}} & \multicolumn{1}{c}{\rotatebox{90}{BNSL-2016}} & \multicolumn{1}{c}{\rotatebox{90}{CPMP-2015}} & \multicolumn{1}{c}{\rotatebox{90}{CSP-2010}} & \multicolumn{1}{c}{\rotatebox{90}{CSP-MZN-2013}} & \multicolumn{1}{c}{\rotatebox{90}{CSP-Minizinc-Time-2016  }} & \multicolumn{1}{c}{\rotatebox{90}{GLUHACK-18}} & \multicolumn{1}{c}{\rotatebox{90}{MAXSAT12-PMS}} & \multicolumn{1}{c}{\rotatebox{90}{MAXSAT15-PMS-INDU}} & \multicolumn{1}{c}{\rotatebox{90}{QBF-2011}} & \multicolumn{1}{c}{\rotatebox{90}{SAT03-16\_INDU}} & \multicolumn{1}{c}{\rotatebox{90}{SAT12-INDU}} & \multicolumn{1}{c}{\rotatebox{90}{SAT18-EXP}} \\ \hline
\multicolumn{1}{l|}{\#I}          & \multicolumn{1}{l|}{1294}        & \multicolumn{1}{l|}{1179}     & \multicolumn{1}{l|}{527}      & \multicolumn{1}{l|}{2024}    & \multicolumn{1}{l|}{4642}        & \multicolumn{1}{l|}{100}                   & \multicolumn{1}{l|}{353}          & \multicolumn{1}{l|}{876}         & \multicolumn{1}{l|}{601}              & \multicolumn{1}{l|}{1368}    & \multicolumn{1}{l|}{2000}          & \multicolumn{1}{l|}{1167}      & \multicolumn{1}{l|}{353}                              \\ \hline
\multicolumn{1}{l|}{\#U} & \multicolumn{1}{l|}{82}          & \multicolumn{1}{l|}{0}        & \multicolumn{1}{l|}{0}        & \multicolumn{1}{l|}{253}     & \multicolumn{1}{l|}{944}         & \multicolumn{1}{l|}{17}                    & \multicolumn{1}{l|}{116}          & \multicolumn{1}{l|}{129}         & \multicolumn{1}{l|}{44}               & \multicolumn{1}{l|}{314}     & \multicolumn{1}{l|}{269}           & \multicolumn{1}{l|}{209}       &   \multicolumn{1}{l|}{67}    \\ \hline
\multicolumn{1}{l|}{\#A}         & \multicolumn{1}{l|}{11}          & \multicolumn{1}{l|}{8}        & \multicolumn{1}{l|}{4}        & \multicolumn{1}{l|}{2}       & \multicolumn{1}{l|}{11}          & \multicolumn{1}{l|}{20}                    & \multicolumn{1}{l|}{8}          & \multicolumn{1}{l|}{6}           & \multicolumn{1}{l|}{29}               & \multicolumn{1}{l|}{5}       & \multicolumn{1}{l|}{10}            & \multicolumn{1}{l|}{31}        & \multicolumn{1}{l|}{37}                              \\ \hline
\multicolumn{1}{l|}{\#F}           & \multicolumn{1}{l|}{138}         & \multicolumn{1}{l|}{86}       & \multicolumn{1}{l|}{22}       & \multicolumn{1}{l|}{86}      & \multicolumn{1}{l|}{155}         & \multicolumn{1}{l|}{95}                    & \multicolumn{1}{l|}{50}          & \multicolumn{1}{l|}{37}          & \multicolumn{1}{l|}{37}               & \multicolumn{1}{l|}{46}      & \multicolumn{1}{l|}{483}           & \multicolumn{1}{l|}{115}       &  \multicolumn{1}{l|}{50}                              \\ \hline
\multicolumn{1}{l|}{C}             & \multicolumn{1}{l|}{600}         & \multicolumn{1}{l|}{7200}     & \multicolumn{1}{l|}{3600}     & \multicolumn{1}{l|}{5000}    & \multicolumn{1}{l|}{1800}        & \multicolumn{1}{l|}{1200}                  & \multicolumn{1}{l|}{5000}          & \multicolumn{1}{l|}{2100}        & \multicolumn{1}{l|}{2100}             & \multicolumn{1}{l|}{3600}    & \multicolumn{1}{l|}{5000}          & \multicolumn{1}{l|}{1200}      & \multicolumn{1}{l|}{5000}    \\
\hline                          
\end{tabular}

\end{document}
