# Supplementary material for: Algorithm Selection on a Meta Level
Source: arXiv:2107.09414 source file (2021-07-20)
Supplement: Supplementary file 3 [file n_par10_level_1.tex]

\begin{tabular}{l||rrrrrrr}
\toprule
Approach &  R2SExp &  R2SPAR10 &     ISAC &     MCC &    PAReg &  SATzilla'11 &   SUNNY \\
Scenario          &         &           &          &         &          &              &         \\
\midrule

ASP-POTASSCO & 3.15 & 2.03 & 1.46 & 5.46 & 2.77 & 2.80 & 1.71\\
BNSL-2016 & \textbf{0.87} & \textbf{0.74} & \textbf{0.86} & 1.41 & \textbf{0.97} & 1.17 & 1.20\\
CPMP-2015 & 1.05 & 1.05 & 1.17 & 1.33 & 1.12 & 1.01 & 1.22\\
CSP-2010 & 1.07 & \textbf{0.87} & 2.69 & \textbf{0.91} & 272.51 & 1.13 & \textbf{0.79}\\
CSP-MZN-2013 & 2.72 & 1.27 & 1.05 & 3.18 & 5.09 & 8.18 & 3.05\\
CSP-Minizinc-Time-2016 & 1.64 & 1.64 & 2.04 & 14.69 & 3.11 & 1.03 & \textbf{0.94}\\
GLUHACK-18 & \textbf{0.95} & \textbf{0.93} & 1.64 & 1.31 & 1.31 & 1.74 & 1.50\\
%MAXSAT-PMS-2016 & 2.72 & 1.27 & 1.05 & 3.18 & 5.09 & 8.18 & 3.05\\
%MAXSAT-WPMS-2016 & 1.20 & 5.44 & 3.84 & 11.1 & 7.83 & 4.44 & 3.37\\
MAXSAT12-PMS & \textbf{0.70} & \textbf{0.77} & \textbf{0.74} & \textbf{0.82} & 1.09 & \textbf{0.70} & \textbf{0.66}\\
MAXSAT15-PMS-INDU & 1.48 & 3.76 & 1.01 & 2.93 & 3.00 & 4.37 & 1.41\\
%MIP-2016 & 1.01 & 1.00 & 1.13 & \textbf{0.99} & 1.00 & \textbf{0.95} & \textbf{0.76}\\
%PROTEUS-2014 & 1.18 & 1.20 & 1.30 & 1.34 & 1.49 & 1.76 & 1.50\\
QBF-2011 & 1.34 & 1.49 & 1.67 & 1.22 & 1.85 & 1.75 & 2.04\\
%QBF-2014 & 1.16 & 1.22 & 1.51 & 1.53 & 1.55 & 1.66 & 1.54\\
%QBF-2016 & \textbf{0.91} & \textbf{0.96} & 1.00 & \textbf{0.88} & 1.09 & 1.20 & 1.09\\
SAT03-16\_INDU & 1.48 & 1.46 & 1.23 & 1.30 & 1.29 & 1.45 & 1.49\\
%SAT11-HAND & 1.50 & 1.92 & 1.47 & 1.51 & 1.91 & 1.92 & 2.62\\
%SAT11-INDU & 1.33 & 1.38 & 1.31 & \textbf{0.89} & 1.48 & 1.00 & 1.43\\
%SAT11-RAND & 1.76 & 1.52 & 6.06 & 4.54 & 2.74 & 11.21 & 6.48\\
%SAT12-ALL & 1.08 & 1.21 & 1.21 & 1.19 & 1.33 & 1.29 & 1.36\\
%SAT12-HAND & 1.38 & 1.27 & 1.28 & 1.83 & 1.89 & 1.64 & 1.56\\
SAT12-INDU & 1.24 & 1.25 & 1.38 & 1.41 & 1.27 & 1.21 & 1.15\\
%SAT12-RAND & 1.01 & 1.15 & 1.08 & 1.12 & 1.60 & 1.49 & 1.30\\
%SAT15-INDU & \textbf{0.73} & \textbf{0.83} & 1.19 & 1.14 & \textbf{0.67} & \textbf{0.68} & \textbf{0.89}\\
SAT18-EXP & \textbf{0.73} & \textbf{0.83} & 1.19 & 1.14 & \textbf{0.67} & \textbf{0.68} & \textbf{0.89}\\
%TSP-LION2015 & 1.14 & 1.05 & 10.86 & 22.55 & 2.00 & 27.62 & 8.00\\
\bottomrule
\end{tabular}
