# Supplementary material for: Algorithm Selection on a Meta Level
Source: arXiv:2107.09414 source file (2021-07-20)
Supplement: Supplementary file 4 [file n_par_10_all_normalized_by_level_0.tex]

\begin{tabular}{l||rrrrrrr|rrrrrrr}
\toprule
\multicolumn{1}{c||}{Level} & \multicolumn{7}{c}{Algorithm Selectors} & \multicolumn{7}{|c}{Algorithm Selector Selectors (Meta)} \\
\toprule
\multicolumn{1}{r||}{\rotatebox{90}{Approach}} &  \multicolumn{1}{c}{\rotatebox{90}{R2SExp}} &  \multicolumn{1}{c}{\rotatebox{90}{R2SPAR10}} &   \rotatebox{90}{ISAC} &    \multicolumn{1}{c}{\rotatebox{90}{MCC}} & \multicolumn{1}{c}{\rotatebox{90}{PAReg}} &  \multicolumn{1}{c}{\rotatebox{90}{SATzilla'11}} &  \rotatebox{90}{SUNNY} &  \multicolumn{1}{c}{\rotatebox{90}{R2SExp}} &  \multicolumn{1}{c}{\rotatebox{90}{R2SPAR10}} &  \multicolumn{1}{c}{\rotatebox{90}{ISAC}} &  \multicolumn{1}{c}{\rotatebox{90}{MCC}} &  \multicolumn{1}{c}{\rotatebox{90}{PAReg}} &  \multicolumn{1}{c}{\rotatebox{90}{SATzilla'11}} &  \multicolumn{1}{c}{\rotatebox{90}{SUNNY}} \\
Scenario         &         &           &        &        &              &        &            &              &          &         &           &                 &           \\
\midrule

ASP-POTASSCO & 0.30 & 0.32 & 0.63 & 0.64 & 0.34 & 0.47 & \textbf{0.17} & 0.26 (6/1) & 0.21 (6/1) & 0.26 (6/1) & 0.37 (3/4) & 0.31 (5/2) & 0.29 (6/1) & 0.26 (6/1)\\
BNSL-2016 & \textbf{0.18} & 0.21 & 0.84 & 0.31 & \textbf{0.18} & \textbf{0.18} & 0.25 & 0.23 (3/4) & 0.21 (4/3) & 0.19 (4/3) & 0.24 (3/4) & 0.23 (3/4) & 0.28 (2/5) & 0.27 (2/5)\\
CPMP-2015 & 0.76 & \textbf{0.69} & 0.90 & 0.85 & 0.78 & 0.70 & 0.94 & 0.78 (4/3) & 0.78 (4/3) & 0.89 (2/5) & 0.81 (3/4) & 0.77 (4/3) & 0.81 (3/4) & 0.89 (2/5)\\
CSP-2010 & 0.13 & 0.15 & 0.31 & 0.80 & 0.25 & 0.13 & 0.34 & \textbf{0.04} (7/0) & 0.10 (7/0) & 0.19 (4/3) & 0.13 (7/0) & 0.46 (1/6) & 0.18 (4/3) & 0.09 (7/0)\\
CSP-MZN-2013 & \textbf{0.11} & \textbf{0.11} & 0.35 & 0.31 & 0.13 & 0.21 & 0.13 & \textbf{0.11} (7/0) & \textbf{0.11} (7/0) & 0.13 (5/2) & 0.15 (3/4) & 0.13 (5/2) & 0.19 (3/4) & 0.14 (3/4)\\
CSP-Minizinc-Time-2016 & 0.43 & \textbf{0.27} & 0.83 & 0.36 & 0.67 & 0.34 & 0.37 & 0.51 (2/5) & 0.51 (2/5) & 0.76 (1/6) & 0.60 (2/5) & 0.67 (2/5) & 0.35 (5/2) & 0.51 (2/5)\\
GLUHACK-18 & 0.43 & 0.46 & 0.69 & 0.41 & 0.46 & 0.42 & 0.51 & \textbf{0.40} (7/0) & 0.45 (4/3) & 0.41 (7/0) & 0.49 (2/5) & 0.57 (1/6) & 0.47 (2/5) & 0.46 (4/3)\\
MAXSAT12-PMS & 0.22 & 0.23 & 0.47 & 0.40 & 0.28 & 0.24 & 0.29 & 0.25 (4/3) & 0.25 (4/3) & 0.20 (7/0) & \textbf{0.19} (7/0) & 0.32 (2/5) & 0.20 (7/0) & 0.21 (7/0)\\
MAXSAT15-PMS-INDU & 0.34 & 0.44 & 0.89 & 1.06 & 0.55 & 0.39 & \textbf{0.24} & 0.36 (5/2) & 0.57 (2/5) & 0.33 (6/1) & 0.39 (5/2) & 0.40 (4/3) & 0.51 (3/4) & 0.26 (6/1)\\
QBF-2011 & 0.21 & 0.20 & 0.36 & 0.35 & 0.18 & \textbf{0.15} & 0.22 & 0.22 (3/4) & 0.22 (3/4) & 0.21 (4/3) & 0.21 (4/3) & 0.29 (2/5) & 0.23 (2/5) & 0.26 (2/5)\\
SAT03-16\_INDU & \textbf{0.71} & 0.76 & 0.98 & 0.99 & 0.77 & 0.82 & 0.82 & 0.92 (2/5) & 0.90 (2/5) & 0.81 (4/3) & 0.79 (4/3) & 0.81 (4/3) & 0.84 (2/5) & 0.86 (2/5)\\
SAT12-INDU & 0.70 & 0.73 & 1.02 & 0.94 & 0.79 & \textbf{0.59} & 0.78 & 0.62 (6/1) & 0.63 (6/1) & 0.75 (4/3) & 0.73 (5/2) & 0.65 (6/1) & 0.65 (6/1) & 0.66 (6/1)\\
SAT18-EXP & 0.61 & 0.68 & 0.62 & 0.65 & 0.64 & 0.59 & 0.63 & 0.66 (1/6) & 0.67 (1/6) & 0.61 (6/1) & 0.58 (7/0) & 0.61 (6/1) & \textbf{0.54} (7/0) & 0.59 (7/0)\\
\bottomrule
\end{tabular}
